# Supplementary material for: Turbo Training with Token Dropout
Source: arXiv:2210.04889 source file (2022-10-10)
Supplement: Supplementary file 1 [file supp.tex]

\documentclass{bmvc2k}

%% Enter your paper number here for the review copy
% \bmvcreviewcopy{622}

%\title{Turbo-charged Training\\ Using Masked Autoencoders}
% \title{Turbo-charged Training with Token Dropout}
\title{Supplementary Material for\\
{\Large Turbo Training with Token Dropout}}
% Enter the paper's authors in order
% \addauthor{Name}{email/homepage}{INSTITUTION_CODE}

\addauthor{Tengda Han}{htd@robots.ox.ac.uk}{1}
\addauthor{Weidi Xie}{weidi@robots.ox.ac.uk}{1,2}
\addauthor{Andrew Zisserman}{az@robots.ox.ac.uk}{1}

% Enter the institutions
% \addinstitution{Name\\Address}
\addinstitution{
 Visual Geometry Group\\
 Department of Engineering Science\\
 University of Oxford\\
}
\addinstitution{
%  MediaBrain\\
Coop.\ Medianet Innovation Center \\ Shanghai Jiao Tong University \\ Shanghai, China
}

\runninghead{Han, Xie, Zisserman}{Turbo Training with Token Dropout}

% Any macro definitions you would like to include
% These are not defined in the style file, because they don't begin
% with \bmva, so they might conflict with the user's own macros.
% The \bmvaOneDot macro adds a full stop unless there is one in the
% text already.

%

\input{sec/def}

\usepackage[svgnames]{xcolor}
\usepackage{caption}
\definecolor{bmvc_blue}{RGB}{0,0,102} 
\captionsetup{margin=3pt , font=small,  labelfont={color=black,bf}, labelsep=period, skip=4pt}

\usepackage{bm}
\usepackage{comment}
\usepackage{bbding}
\usepackage{comment}
\usepackage{amssymb}
\usepackage{multirow}
\usepackage{booktabs}
\usepackage{subfigure}
\usepackage{todonotes}
\usepackage{graphicx}
\usepackage[font={small}]{caption}
\usepackage{comment}
\usepackage{tabu}
%------------------------------------------------------------------------- 
% Document starts here
\begin{document}

\maketitle

\input{sec/08-supp}

% \clearpage
\bibliography{bib/shortstrings,bib/vgg_local,bib/vgg_other}
\end{document}
