# Supplementary material for: Turbo Training with Token Dropout
Source: arXiv:2210.04889 source file (2022-10-10)
Supplement: Supplementary file 2 [file supp_alignment.tex]

\begin{table}[h]
    \centering
    \small
    \begin{tabu}{c|c|c|c|c}
        \hline
           Method & Arch. & Pretrain Data & Temporal R.F. & R@1 \\ \hline
           CLIP~\cite{Radford21} & ViT-B-32 & YFCC & 1s & 16.8 \\
           CLIP~\cite{Radford21} & ViT-B-16 & YFCC & 1s & 22.0 \\
           MIL-NCE~\cite{Miech20} & S3D-G & HTM & 1s & 31.3 \\
           \rowfont{\color{gray}}
           TAN$^{*}$~\cite{Han22TAN} & S3D-G \& TFM  & HTM & 64s & 49.4 \\ 
           NCE with TAN$^{\dag}$~\cite{Han22TAN} & S3D-G & HTM-AA  & 1s. & {33.6} \\
           \hline
           Ours (m=0.75, r=0.25) & ViT-B-16 & HTM-AA & 1s & \textbf{36.7} \\
        \hline
    \end{tabu}
    \caption{
    Zero-shot text-visual alignment results on HTM-Align dataset. 
    We adopt the same setting as~\cite{Han22TAN} and report Recall@1 as the metric.
    $*$: result from TAN is not directly comparable
    because their model contains transformers (TFM) on S3D-G features that takes a much longer temporal context for the temporal alignment task. This table provides additional comparisons and details over Table~3 (right) in the main paper.
    $\dag$: we train the NCE loss on HTM-AA for the same duration (approx. 60h) for a fair comparison. 
    }
    \label{tab:supp_pretrain}
    \vspace{-5mm}
\end{table}
